# Supplementary material for: Benchmarking Geospatial Foundation Models under Calibrated Label Errors
Source: arXiv:2611.30215 source file (2026-11-23)
Supplement: Supplementary file 1 [file supp_refs.tex]

\expandafter\def\csname sref@tab:supp-calibration\endcsname{1}
\expandafter\def\csname sref@sec:supp-calibration\endcsname{A}
\expandafter\def\csname sref@fig:supp-mechanics\endcsname{1}
\expandafter\def\csname sref@tab:supp-realizations\endcsname{2}
\expandafter\def\csname sref@tab:supp-omadj\endcsname{3}
\expandafter\def\csname sref@tab:supp-acceptance\endcsname{4}
\expandafter\def\csname sref@sec:supp-acceptance\endcsname{B}
\expandafter\def\csname sref@sec:supp-grid\endcsname{C}
\expandafter\def\csname sref@sec:supp-collapsed\endcsname{D}
\expandafter\def\csname sref@sec:supp-perclass\endcsname{E}
\expandafter\def\csname sref@sec:supp-boundary\endcsname{F}
\expandafter\def\csname sref@tab:supp-main\endcsname{5}
\expandafter\def\csname sref@fig:supp-dose\endcsname{2}
\expandafter\def\csname sref@sec:supp-ablation\endcsname{G}
\expandafter\def\csname sref@fig:supp-typedrop\endcsname{3}
\expandafter\def\csname sref@sec:supp-budget\endcsname{H}
\expandafter\def\csname sref@tab:supp-grid-burn\endcsname{6}
\expandafter\def\csname sref@tab:supp-grid-flair\endcsname{7}
\expandafter\def\csname sref@tab:supp-collapsed\endcsname{8}
\expandafter\def\csname sref@tab:supp-collapsed-sens\endcsname{9}
\expandafter\def\csname sref@tab:supp-perclass\endcsname{10}
\expandafter\def\csname sref@tab:supp-perclass-drop\endcsname{11}
\expandafter\def\csname sref@tab:supp-boundary\endcsname{12}
\expandafter\def\csname sref@sec:supp-fliprate\endcsname{I}
\expandafter\def\csname sref@sec:supp-stats\endcsname{J}
\expandafter\def\csname sref@tab:supp-mlr\endcsname{13}
\expandafter\def\csname sref@fig:supp-budget\endcsname{4}
\expandafter\def\csname sref@tab:supp-ablation\endcsname{14}
\expandafter\def\csname sref@fig:supp-frozen\endcsname{5}
\expandafter\def\csname sref@tab:supp-frozen\endcsname{15}
\expandafter\def\csname sref@tab:supp-budget\endcsname{16}
\expandafter\def\csname sref@tab:supp-breakeven\endcsname{17}
\expandafter\def\csname sref@tab:mem\endcsname{18}
\expandafter\def\csname sref@fig:supp-er\endcsname{6}
\expandafter\def\csname sref@fig:supp-mem\endcsname{7}
\expandafter\def\csname sref@sec:supp-stretch\endcsname{K}
\expandafter\def\csname sref@tab:supp-sen1floods\endcsname{19}
\expandafter\def\csname sref@sec:supp-hardware\endcsname{L}
\expandafter\def\csname sref@tab:supp-stretch\endcsname{20}
\expandafter\def\csname sref@tab:supp-blocks\endcsname{21}
\expandafter\def\csname sref@fig:supp-roster\endcsname{8}
\expandafter\def\csname sref@tab:supp-models\endcsname{22}
\expandafter\def\csname sref@tab:supp-hardware\endcsname{23}
\expandafter\def\csname sref@tab:supp-manifest\endcsname{24}
\expandafter\def\csname sref@tab:supp-hwmix\endcsname{25}
